# Supplementary material for: Boosting Graph Search with Attention Network for Solving the General Orienteering Problem
Source: arXiv:2109.04730 source file (2021-09-10)
Supplement: Supplementary file 1 [file appendix.tex]

\section*{appendix}
In this section, we present the necessary details about our empirical studies. 
Our experiment is conducted on a single machine with an Intel Xeon E5 and an NVIDIA TITAN GPU. We implement our neural networks by Pytorch. 

Our code including  benchmarks is publicly available in \href{https://anonymous.4open.science/repository/7cb20ede-b50e-4a9a-99a5-e3c3626bf1a1/}{\textbf{[code]}}. The testing data is available in \href{https://anonymous.4open.science/repository/7cb20ede-b50e-4a9a-99a5-e3c3626bf1a1/data/}{\textbf{[data]}}.
\subsection*{Details of Baselines}
In this subsection, we present the implementation details of some of the baselines in \secref{sec:baselines}.
\begin{itemize} %[leftmargin=*]
	\item \textit{Gurobi:}  This baseline is an exact method solved by the Gurobi optimizer\cite{optimization2014inc}.
	%, which solves the mix integer problem corresponding to each instance and produces the optimal results. It is intractable for problem size more than 20.
	\item \textit{Compass:}  This is a state-of-the-art Genetic Algorithm for solving the OP\cite{kobeaga2018efficient}.
	\item \textit{Random:}  At each state, a node is randomly selected from the rest nodes.
	\item \textit{Tsili:}  \citet{tsiligirides1984heuristic} propose a manual defined function to compute node selection probability in each state.
	\item \textit{AN-dqn:} At each step, the node v with the highest action value $q(s, v; \theta)$ will be selected. The beam search version of this baseline is the step-by-step beam search with the learned heuristic.
	\item \textit{AN-a2c:} We apply the advantage Actor-Critic algorithm to learn the policy of each state. For each state s,  an attention network proposed in \secref{sec:model} is shared for the actor-network and the critic-network to obtain node embeddings. In the actor-network, we then project the embedding of each node to get the logit by a linear combination, followed by a softmax operator to get the normalized selection probability. In the critic-network, we map the sum of embeddings to the estimated value by another linear layer.
	\item \textit{AN-at:} \citet{kool2018attention} propose an attention-based encoder-decoder architecture to solve the routing problem and train it using policy gradient with the deterministic greedy rollout baseline. As the original encoder used in \cite{kool2018attention} can only support the input of nodes' coordinates, we replace it by the attention network proposed in \secref{sec:model}.
	\item \textit{AN-pt:} \citet{nazari2018reinforcement} design an encoder-decoder based model to perform routing by decoding the encoded embeddings of nodes via pointer network\cite{vinyals2015pointer}. As the original encoder used in \citet{nazari2018reinforcement} can only support nodes' coordinates as input, we use our attention network as the encoder.
	\item \textit{CS(K, $\tau$):}  This approach refers to the cost-level beam search with learned heuristic as the score function. $K$ and $\tau$ represent the beam size and cost interval, respectively.
\end{itemize}
\vpara{Hyperparameters.} For the implementations of the NN-based baselines, we set the same hyperparameters. In the experiment, we conduct the training procedure 5 times and report the result from the model with the best performance on 200 validation instances.

\begin{table}[ht]
	\centering
	
	\begin{tabular}{|l|c|c|c|}
		\hline
		\textbf{Hyperparameter} &value &Hyperparameter &value \\ \hline
		\textbf{\#head in GAT} &20 &\textbf{\#head in TEL} &8 \\ \hline
		\textbf{\#TEL} &4&\textbf{hidden size} &64 \\ \hline
		\textbf{learning rate}&1e-3&\textbf{optimizer}&Adam \\ 
		\hline
	\end{tabular}
\caption{Hyperparameters for NNs.}
\end{table}
\vpara{Beam Search.}For the beam search versions of  $Tsili, AN-a2c, AN-at, AN-pn$, we set the heuristic function as the  accumulation of log-likelihood probabilities $\sum_i logp_i$. For the beam search version of $AN-dqn$, we set the heuristic function the same as \eqref{eq:f}.

\vpara{Tsili.}
 The heuristic function to compute $p(v|s)$ used by \citet{tsiligirides1984heuristic} is a formula with multiple terms to compute the probability that a node should be expanded, but by tuning the weights the form with only one simple term works best, showing the difficulty of manually defining a good probability distribution. We use the following formula to compute such probability:
\begin{equation}
f(v, P) = \left(\frac{R_v}{C_{last(P),v}}\right)^4.
\end{equation}
Let $S$ be the set with $\min(4, n - (t - 1))$ unvisited nodes with maximum score $f_v$. Then the node probabilities $p_v$ at time $t$ are defined as
\begin{equation}
\label{dec:probabilities_tsili}
p_v = p_{{\theta}}(v|s) =  \begin{cases}
\frac{f_v}{\sum_{w \in S}{f_w}} & \text{if } v \in S \\
0 & \text{otherwise.}
\end{cases}
\end{equation}
\vpara{AN-a2c.}
We apply the advantage Actor-Critic algorithm to learn the policy of each state. For each state s,  an attention network proposed in \secref{sec:model} is shared for the actor-network and the critic-network to obtain node embeddings $\{h_{v_1}, h_{v_1}, ..., h_{v_M}\}$. In the actor network, we then project the embedding of each node to get the logit by a linear combination, followed by a softmax operator to get the normalized selection probability $p(v|s) = softmax(U\cdot h_v)$. In the critic network, we map the sum of embeddings to the estimated value by another linear layer, $V(s) = W \cdot \sum_v h_v$. $U$ and $V$ are learnable variables.

For notation convenience, we define $\theta_1$ as the parameters of actor network, and $\theta_2$ as the parameters of critic networks. The loss function is set as:
\begin{eqnarray}
loss(\theta_1)=\mathbb{E}[-log(p(v_t|s_t) (V(s_t)-V(s_{t+1})-r_{t+1})]\\
loss(\theta_2)=\mathbb{E}[(V(s_t)-V(s_{t+1})-r_{t+1})^2]\\
loss(\theta_1, \theta_2) = loss(\theta_1) + 0.5\cdot loss(\theta_2)
\end{eqnarray} 

\vpara{AN-at}. 
\citet{kool2018attention} propose an attention-based encoder-decoder architecture to solve the routing problem and train it using policy gradient with the deterministic greedy rollout baseline. As the original encoder used in \cite{kool2018attention} can only support the input of nodes' coordinates, we replace it by the attention network proposed in \secref{sec:model}. 

More specifically, in the decoding step, we set the context for the decoder input at step $t$ is the current/last location $last(P)$ and the remaining travel cost $T-cost(P)$. The context is defined as:
\begin{equation}
\mathbf{h}_{(c)}^{(N)} = \begin{cases}
[\bar{\mathbf{h}'} , \mathbf{h}'_{last(P)} , T-cost(P) ] & t > 1 \\
[\bar{\mathbf{h}'} , \mathbf{h}'_0 ,T-cost(P) ] & t = 1.
\end{cases} \\
\end{equation}
where $\mathbf{h}'_v$ denotes the node $v$'s embedding, $\bar{\mathbf{h'}}$ represents the average node embedding and $\mathbf{h'}_0$ is a learnable vector as the decoder initial input. All visited nodes in the decoding are masked.

\vpara{AN-pn.}  \citet{nazari2018reinforcement} design an encoder-decoder based model to perform routing by decoding the encoded embeddings of nodes via pointer network\cite{vinyals2015pointer}. As the original encoder used in \citet{nazari2018reinforcement} can only support nodes' coordinates as input, we use our attention network as the encoder.

At decoder step $i$, we use a context-based attention mechanism, which extracts the relevant information from the inputs using a variable-length alignment vector $a_t$. 

We let ${\mathbf{h'_{t,v}}}$ be the embedded input of node $v$ at step $t$, and $h_t\in \mathbb{R}^D$ be the hidden state of the LSTM cell at decoding step $t$. The alignment vector $a_t$ is then computed by
\begin{eqnarray} 
a^t = a_t(h'_{t,v} ,  h_t) = \text{softmax} \left(u_t\right)\label{eq:vrp:align}
\\u_t^i = v^T_a\tanh\left( W_a [\bar{h'}_{t,v}||h_t ]\right)
\end{eqnarray}
We obtain the conditional probabilities by combining the context vector $c_t$, as follows:
\begin{equation}
c_t = \sum_{i=1}^{M} a_t^i \bar{h'}_{t,v}, \label{eq:vrp:ct}
\end{equation}
with the embedded inputs, and then use softmax function to normalize the values:
\begin{eqnarray}
P(v_t|s_{t}) = 
\text{softmax}(\tilde{u}_t^i) \\
\tilde{u}_t^i = v^T_c\tanh\left(W_c [\bar{h'}_{t,v}||c_t]\right) \label{eq:vrp:probct}.
\end{eqnarray}
In \eqref{eq:vrp:align}--\eqref{eq:vrp:probct}, $v_a$, $v_c$, $W_a$ and $W_c$ are trainable variables.
